# Supplementary material for: On the Complexity of Telephone Broadcasting: From Cacti to Bounded Pathwidth Graphs
Source: arXiv:2501.12316 source file (2025-02-11)
Supplement: Supplementary file 1 [file pseudocode.tex]

%-----------algorithms--------

\begin{algorithm}
\caption{\singlefunc{$G, s$}}\label{alg:single_source_solver}
\hspace*{\algorithmicindent} \textbf{Input:} A graph $G$ and a source vertex $s$.\\
\hspace*{\algorithmicindent} \textbf{Output:} The broadcast time for a multi-broadcast scheme (with $k=2$) of %the algorithm on 
$G$ with source vertex $s$.
\begin{algorithmic}[1]
\STATE $B \gets \{\}$
\FOR{each connected component $C_i \in G \setminus \{ s \}$}
    \IF{$C_i$ contains a single neighbor $v_i$ of $s$}
        \STATE $b$ $\gets$ \singlefunc{$C_i, v_i$}
    \ELSIF{$C_i$ contains two neighbors $v_i$ and $u_i$ of $s$}
        \STATE $b$ $\gets$ \doublefunc{$C_i, v_i, u_i$}
    \ENDIF
    \STATE $B$ $\gets$ $B$ $\cup$ \{b\}
\ENDFOR
\STATE Sort $B$ in non-increasing order.
% \STATE $\textit{max\_time} \gets 0$
% \STATE $\textit{num\_components} \gets \text{length}(B)$
\STATE $\textit{max\_time} = \max_{i\in [|B|]} (i+B[i])$
% \FOR{$i$ in $\textit{num\_components}$}
%     \STATE $\textit{total\_time} \gets (i + 1) + B[i]$
%     \STATE $\textit{max\_time} \gets \max(\textit{max\_time}, \textit{total\_time})$
% \ENDFOR
\STATE \textbf{return} $\textit{max\_time}$
\end{algorithmic}
\end{algorithm}

\todo{update algorithm 2 or remove it. }
\begin{algorithm}
\caption{\doublefunc{$G, s_1, s_2$}}\label{alg:double_source_solver}
\hspace*{\algorithmicindent} \textbf{Input:} A graph $G$ and two source vertices $s_1$ and $s_2$.\\
\hspace*{\algorithmicindent} \textbf{Output:} The total broadcasting time of the algorithm for $G$ given that $s_1$ and $s_2$ are informed and they have a unique path to each other. 

\begin{algorithmic}[1]
\STATE $\textit{min\_broadcast\_time} \gets \infty$
\FOR{each edge $e$ in the unique path between $s_1$ and $s_2$}
    \STATE $G_e \gets G \setminus \{e\}$
    \STATE $G_1 \gets G_e \cap \text{vertices reachable from } s_1$
    \STATE $G_2 \gets G_e \cap \text{vertices reachable from } s_2$
    \STATE $T_s \gets $\singlefunc{$G_1, s_1$}.
    \STATE $T_d \gets $\singlefunc{$G_2, s_2$}.
    \STATE $\textit{broadcast\_time} \gets \max(T_s, T_d)$.
    \STATE $\textit{min\_broadcast\_time} \gets \min(\textit{min\_broadcast\_time}, \textit{broadcast\_time})$.
\ENDFOR
\STATE \textbf{return} $\textit{min\_broadcast\_time}$
\end{algorithmic}
\end{algorithm}
