# Supplementary material for: On the Complexity of Telephone Broadcasting: From Cacti to Bounded Pathwidth Graphs
Source: arXiv:2501.12316 source file (2025-02-11)
Supplement: Supplementary file 2 [file A-Appendix-2approx.tex]

\newpage

\section{Appendix: Details of Section~\ref{sec:2approx}}
\label{appendix2approx}
\markboth{Appendix A}{Appendix A}
\FloatBarrier

\subsection{\ouralgo Algorithm}
