# Supplementary material for: On the Complexity of Telephone Broadcasting: From Cacti to Bounded Pathwidth Graphs
Source: arXiv:2501.12316 source file (2025-02-11)
Supplement: Supplementary file 3 [file B-Appendix-hardness.tex]

\newpage
\section{Appendix: Details of Section~\ref{sec:hardness}}
\label{appendix-hardness}
\markboth{Appendix B}{Appendix B}
\FloatBarrier

% \tododone{headings of these pages are not correct.}

\subsection{Hardness of the \tislong Problem}
\FloatBarrier

\subsection{Hardness of the \dsprlong Problem}
\FloatBarrier

\subsection{Hardness of \telebg in \Flower Graphs}
\FloatBarrier
