# Supplementary material for: On the Complexity of Telephone Broadcasting: From Cacti to Bounded Pathwidth Graphs
Source: arXiv:2501.12316 source file (2025-02-11)
Supplement: Supplementary file 4 [file C-Appendix_constant.tex]

\newpage
\section{Appendix: Details of Section~\ref{sec:pathwidth-approx}}
\markboth{Appendix C}{Appendix C}
\label{appendix-constant}
\FloatBarrier
