# Supplementary material for: On the Complexity of Telephone Broadcasting: From Cacti to Bounded Pathwidth Graphs
Source: arXiv:2501.12316 source file (2025-02-11)
Supplement: Supplementary file 7 [file 3-broadguesshard.tex]

\subsection{Hardness of \telebg in \Flower Graphs}
\FloatBarrier
